# Supplementary material for: A Technical Framework for Musical Biofeedback in Stroke Rehabilitation
Source: arXiv:2012.00323 source file (2020-12-01)
Supplement: Supplementary file 1 [file Supplementary_Material_1_-_Interface_Structure.pdf]

**The JUCE interface is divided into three tabs to control sensor interfacing, music generation and the biofeedback configuration.**

**SENSOR INTERFACING CONTROLS**

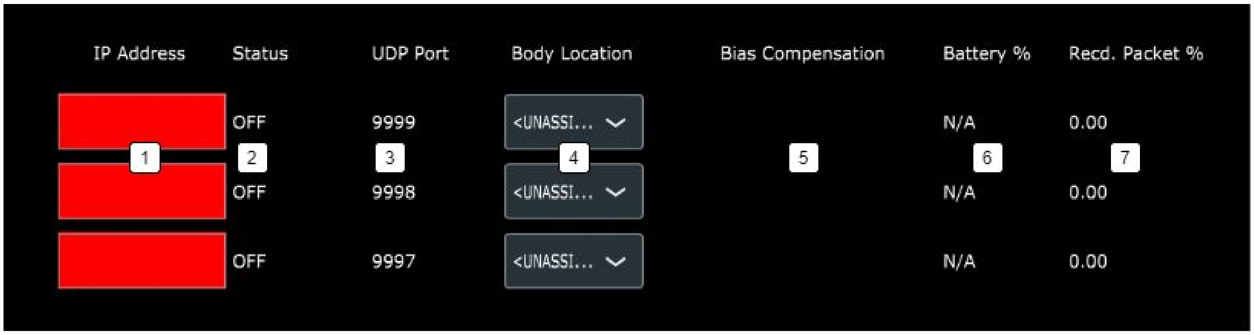


1 - Sensor IP address entry box for bidirectional verification.
2 - Sensor online status.
3 - Local UDP port to receive packets from that sensor.
4 - Assigned body location of sensor.
5 - IMU bias calibration compensation button (appears when sensor is online).
6 - Sensor battery charge level.
7 - Percentage of biofeedback callbacks over the past two seconds where new OSC packets were received. Serves as an indicator of connection health (~50% or above is good).

*(next page)*

## MUSIC GENERATION CONTROLS

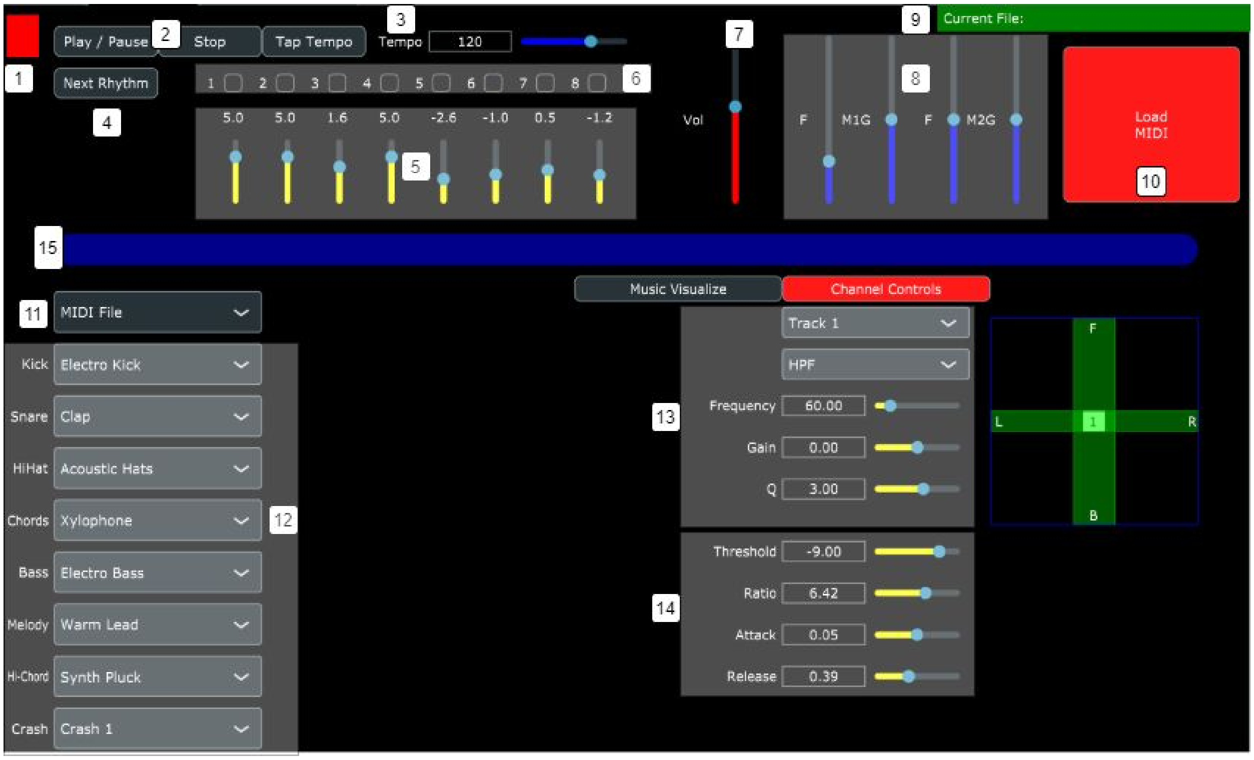


1 - Indicates whether required sensor(s) for presently chosen training exercise is/are online AND properly assigned to body parts (turns green if true).
2 - Music playback controls: Play/pause and stop playback (reset to beginning of song file).
3 - Tempo controls - Slider in beats per minute OR button to manually tap beat rate.
4 - Change playback to next music style (list appears when playback starts).
5 - Individual musical instrument track level adjustment (+/- 10dB).
6 - Individual instrument track mute / unmute.
7 - Master volume level.
8 - Master equalizer frequency and gain controls (Q fixed).
9 - Name of currently loaded MIDI song file.
10 - Browse computer for a MIDI song file (opens window).
11 - Playback mode - External MIDI file or inbuilt MIDI
12 - Change instrument variant for each track
13 - Track channel equalizer controls
14 - Track channel compressor controls
15 - Song progress bar

## MUSICAL BIOFEEDBACK CONTROLS

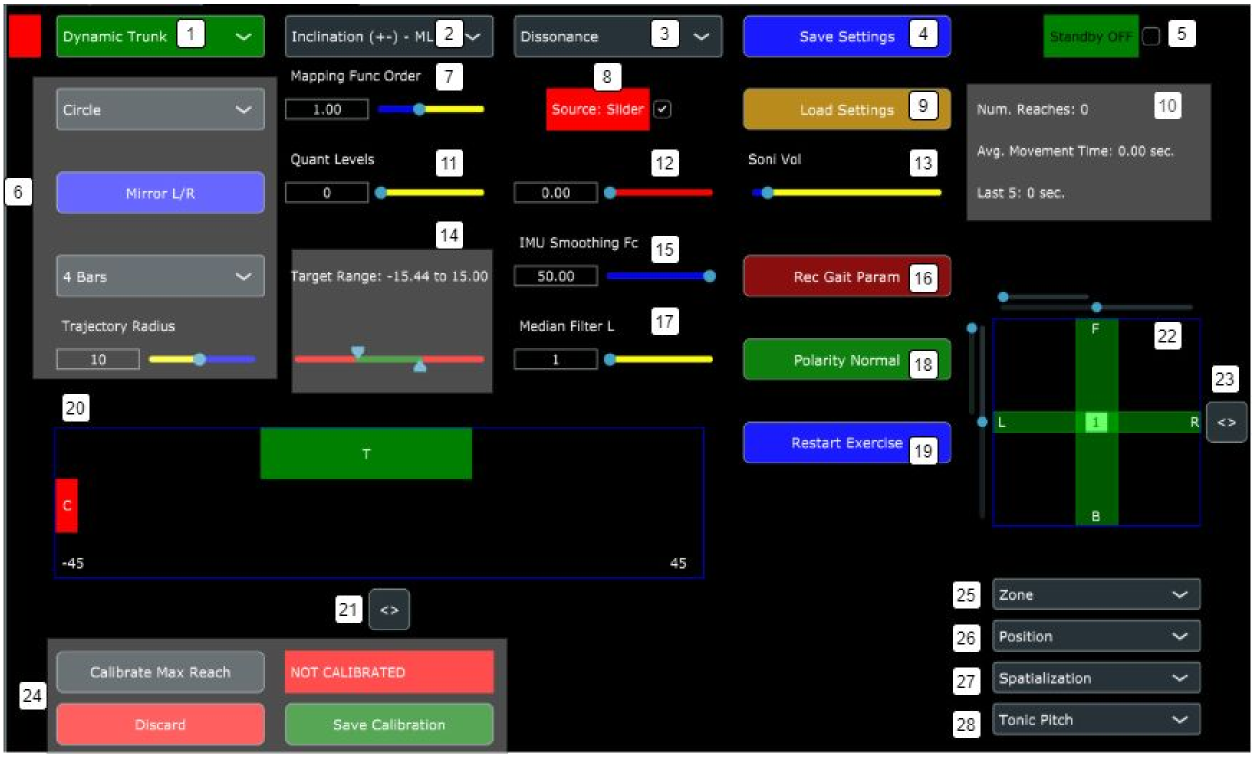


1 - Training exercise mode - static balance, dynamic balance, STS, gait.
2 - 1D MBF - Selected movement parameter.
3 - 1D MBF - Selected musical biofeedback strategy.
4 - Save system settings snapshot.
5 - Standby mode - toggle biofeedback on and off
6 - Exercise-specific controls (change depending on [1])
7 - 1D mapping function order - governs rate of change of biofeedback intensity.
8 - Switches 1D feedback mode between sensor and manual slider (for testing).
9 - Load system settings snapshot.
10 - Movement repetition information display.
11 - Number of feedback quantization levels (0 = continuous).
12 - Manual feedback testing slider (visible when [8] is in slider mode).
13 - Volume control for synthesized sonification strategies.
14 - 1D target range control and display - minimum and maximum bound.
15 - IMU signal smoothing filter cutoff frequency (Hz).
16 - Start or stop session time series logging.
17 - IMU signal median filter length (samples).
18 - Invert 1D feedback polarity.
19 - Reset repetition counts and information.

20 - 1D real-time performance visualizer.
21 - Enlarge [20] to fill the screen.
22 - 2D projection angle visualizer and controls.
23 - Enlarge [22] to fill the screen.
24 - Movement parameter calibration controls.
25 - 2D projection feedback variable - zone / task-based / anticipated distance error
26 - 2D projection feedback variable - position / velocity
27 - 2D projection auditory feedback strategy - ML direction
28 - 2D projection auditory feedback strategy - AP direction

**EXERCISE-SPECIFIC CONTROLS - STS**

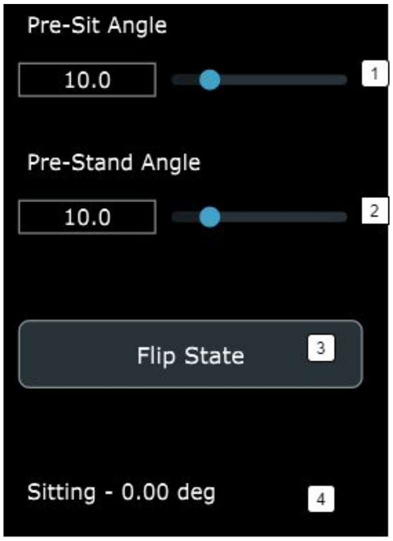


1 - Trunk forward flexion angle to trigger SIT cue.
2 - Trunk forward flexion angle to trigger STAND cue.
3 - Switch presently detected patient state (SITTING to STANDING or vice versa).
4 - Status Monitor.

**EXERCISE-SPECIFIC CONTROLS - DYNAMIC BALANCE**

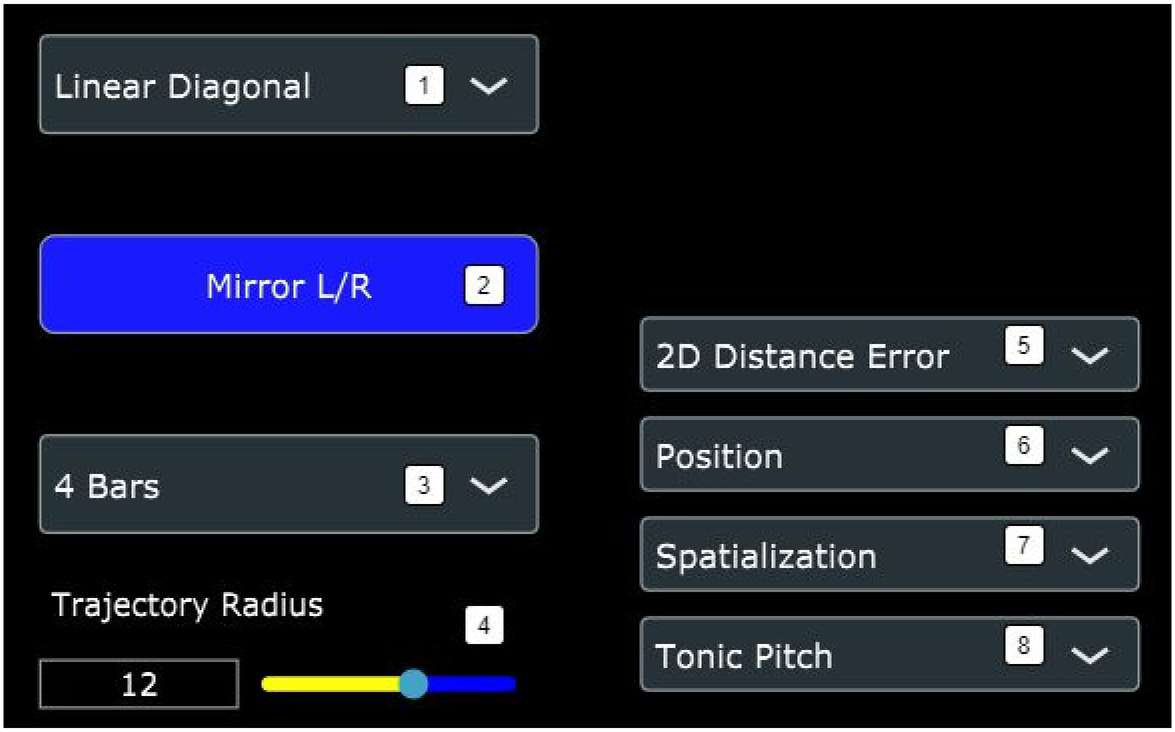


1 - Change trajectory shape.
2 - Mirror trajectory direction in left-right direction.
3 - Change time taken for trajectory cycle completion (in terms of musical measures).
4 - Change trajectory amplitude in degrees of trunk inclination.
5 - Change dynamic tracking feedback variable (zone / task / 2D distance error)
6 - Change feedback variable #2 - position / velocity
7 - Change ML directional feedback strategy
8 - Change AP directional feedback strategy

**EXERCISE-SPECIFIC CONTROLS - GAIT**

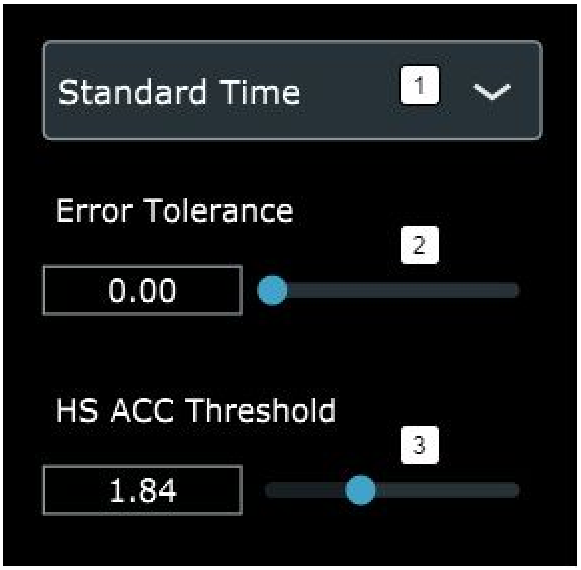


1 - Desired step frequency relative to music: Standard time = 1 step per beat // Half time = 1 step per 2 beats
2 - Error tolerance as a percentage of step interval duration, below which no negative feedback is triggered for step frequency matching interaction.
3 - Accelerometer threshold for algorithmic step detection (may need adjustment depending on gait properties of patient)
