# Supplementary material for: A Technical Framework for Musical Biofeedback in Stroke Rehabilitation
Source: arXiv:2012.00323 source file (2020-12-01)
Supplement: Supplementary file 2 [file Supplementary_Material_2_-_Technical_Evaluation.pdf]

In all experiments, the software was run on a Dell Inspiron 15 7000 Windows laptop with an i7 processor and 16 GB RAM running at 1.8 GHz (4 logical cores). A  USB-connected Focusrite 18i8 audio interface was used for audio output, which was auditioned through a pair of Beyerdynamic DT-880 Pro headphones.

## Sensor Range

The purpose of this test was to study the effect of sensor distance on packet reception efficiency in an indoor environment. The percentage of received OSC packets in a short time interval serves as a good indicator of useful sensor range, providing valuable reference information when using the equipment in real-life environments (e.g. large wards). It is acknowledged that WiFi interference and other signal obstacles vary considerably among buildings and indoor locations, but this evaluation was restricted to a single indoor environment where all factors but sensor distance were kept constant for the experiment duration.

*Experiment*

Setup: The biofeedback application was set up on a Dell laptop placed in the corner of a large furnished room. The laptop itself received its internet connection from a mobile phone hotspot. This connection was shared with a single M5Stack sensor, which transmitted data packets over it at a sampling rate of 125 Hz, while the receiver callback in the application operated at 100 Hz.

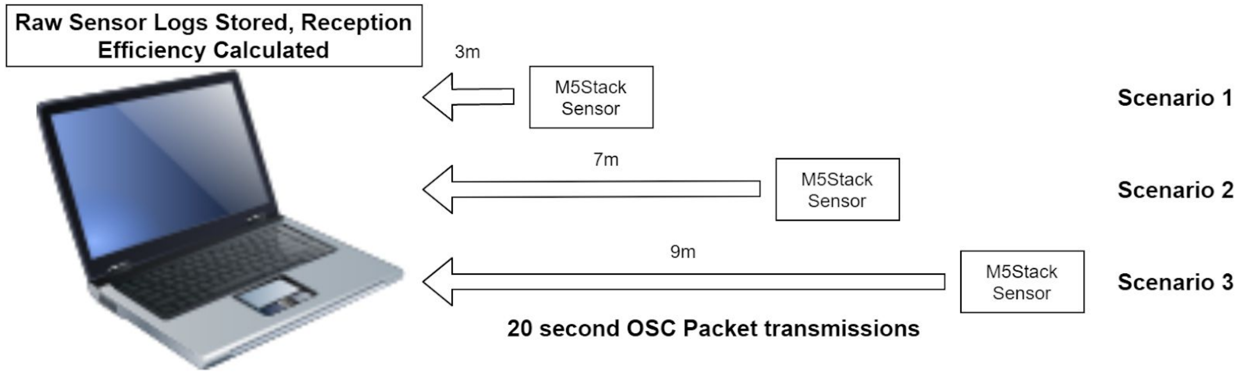


Procedure: Three sensor distances were chosen based on the ergonomics of the selected room:

Scenario 1: 3 meters, direct line-of-sight between sensor and laptop.
Scenario 2: 7 meters, direct line-of-sight between sensor and laptop.
Scenario 3: 9 meters direct distance, but with a wall corner impeding the direct line-of-sight. (WORST CASE SCENARIO)

The sensor was placed on a chair at these measured distances, and raw sensor data logs were stored over a 20 second duration for each location.
The procedure is shown in the figure.

Results: The percentage of receiver callbacks with new OSC packets was calculated from the logs for each distance. The results are as follows:
Scenario 1: 96.35%
Scenario 2: 96.10%
Scenario 3: 82.5%

**Computational Efficiency**

*Experimental Setup*

A standard metric for computational load of a program is % Processor Time. For Windows, this is defined as " the percentage of elapsed time that the processor spends to execute a non-idle thread" 1, in this case the biofeedback application. It is expressed relative to the total available processing capability, i.e. over a baseline of 100% x  no. of logical cores. It was measured in this case using the Windows Performance Monitor (PerfMon), where it is possible to monitor any Windows process and log recorded processor time at 1 sec intervals (fastest possible).

*Procedure*

Music-Only
In these scenarios, no sensors were connected, hence the program automatically skipped the entire MBF callback. A temporally uniform piece of music (single isochronous note over fixed chords) was played back in each of the three styles (Dance, Reggaeton, Slow Rock) at the tempo extremes (60 BPM, 150 BPM). Logs of 100 seconds in length were recorded in PerfMon and imported into MATLAB for analysis.

Worst-Case
The computationally most intense music-only scenario was used in the final CPU stress test, where it was combined with the most complex biofeedback interaction (*dynamic balance training with 2D feedback and performance visualization, session logging enabled*) and a similar logging and analysis was carried out. The CPU Usage % of the entire application in Windows Task Manager was also monitored.

*Results*

Music-Only
The recorded logs were imported into MATLAB and the time series of processor time (100 seconds each) were compared using a box plot, shown in Fig. 1.

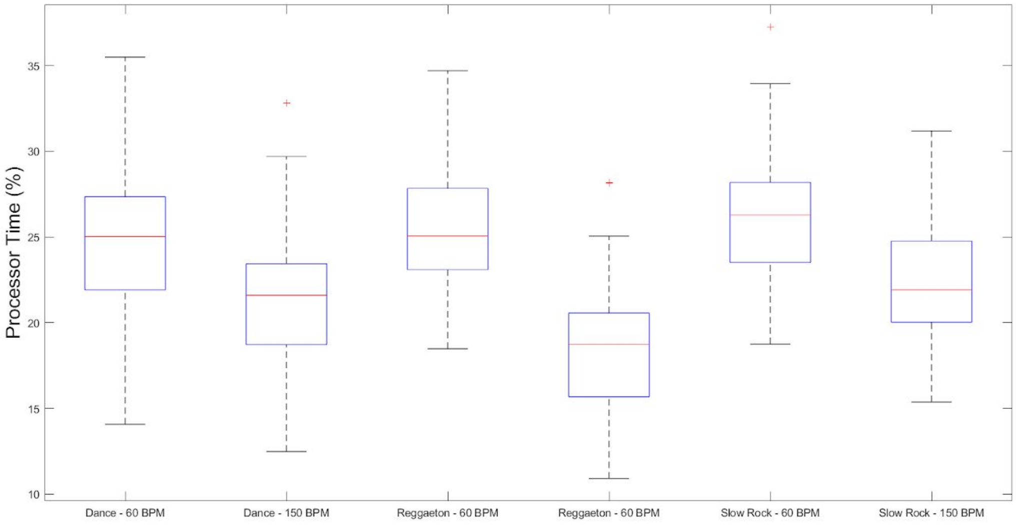


Figure 1: Box plot of % Processor Time logs for all 6 test scenarios (the central mark indicates the median, and the bottom and top edges of the box indicate the 25th and 75th percentiles, respectively. The whiskers extend to the most extreme data points not considered outliers, and the outliers are plotted individually using the '+' symbol.).

It is interesting to note that for each of the styles, the lower tempo extreme is more computationally intensive than the higher, although the opposite would be expected considering the higher frequency of MIDI events to be handled on average. Despite the low temporal resolution of the log, there is considerable variability in the readings and outlier spikes can be seen for some of the scenarios. In terms of mean processor time (%), the Slow Rock - 60 BPM scenario is the most computationally intensive of the tested scenarios.

Worst-Case

The results over 100 seconds are provided here. Fig. 2 depicts the time series of measured % Processor Time.

% Processor Time: 28.91 +/-  4.09 % (Peak: 40.80 %)

Peak CPU Usage (Windows Task Manager): 11.1%

Memory Usage: 157.0 MB

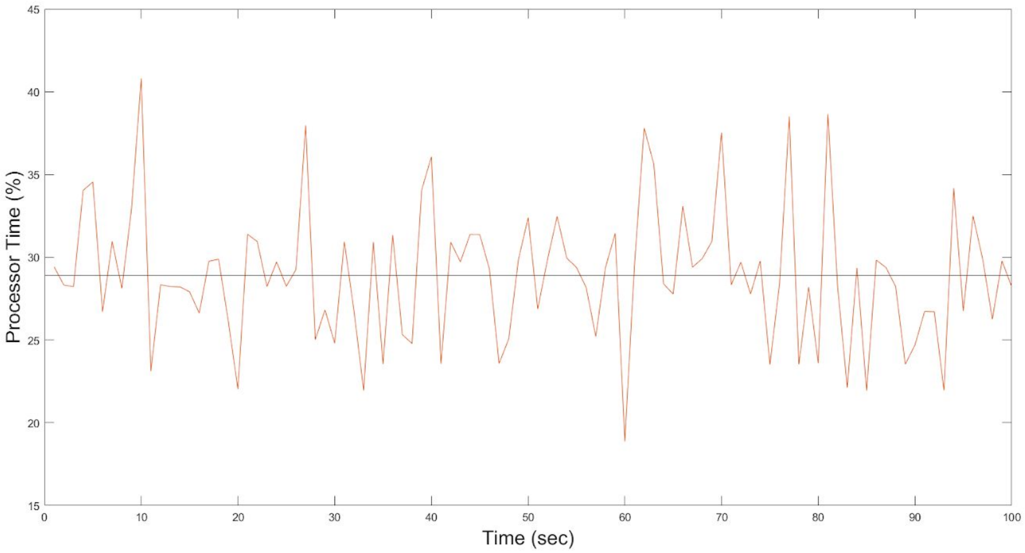


With four logical cores, the Peak % Processor Time and Peak CPU Usage correspond well with each other, although not perfectly as they poll the processor at different instants. No audio dropouts were observed at any moment.

*Discussion*

Overall, the application was seen to perform seamlessly and in a lightweight manner despite having its most computationally complex functional elements running simultaneously. The maximum measured CPU usage was 11.1%, which means that it can run on most modern personal computers in the clinical environment, and, with appropriate optimizations, has the potential to be ported to mobile devices. Moreover, there is ample computational headroom to integrate more complex audio synthesis and processing algorithms, as well as superior sensor fusion-based movement parameter measures. The memory consumption is also modest, implying that heavier hi-res audio samples can be used for superior music generation in future versions.  The variability in the log files is likely due to their low temporal resolution as well as the variations in CPU load at polling instants to the different callback frequencies of the various functional elements. Future studies should carry out performance benchmarks on different systems and in the presence of varying levels of background CPU activity to gauge their effect on the audio output of the application.

**<u>Biofeedback Loop Delay</u>**

*Experimental Setup [Q: Should I redo foot strike? Nothing has changed since the last version]*

- Foot Strike [from thesis version]: The foot strike drum trigger sonification strategy was chosen in the biofeedback application for this measurement, with two separate foot-mounted M5Stack sensors. A handheld mobile recorder was used to record the

sound of the feet physically striking the floor, while a simultaneous mono recorder track in REAPER was set up to capture the triggered drum sounds from the WASAPI driver (Windows Audio Stack).
- Trunk Angle: The bell trigger was used as an impulsive feedback strategy, with all sequenced music tracks muted. The M5Stack sensor was kept upright on a horizontal table, and a similar WASAPI recorder was set up in REAPER to capture the application audio output.

*Procedure*

The WASAPI and mobile recorder simultaneously recorded a sine burst from a loudspeaker to synchronize biofeedback and phone recordings for subsequent analysis. The individual procedures are as follows:
- Foot Strike: 19 steps were taken around the room, while the handheld mobile recorder captured physical heelstrike events as audio signals, and the REAPER recorder captured the triggered drum output of the biofeedback application.
- Trunk Angle: The feedback was triggered by using mouse clicks on the MBF interface to abruptly change the target inclination from the upright position. A mobile recorder was placed next to the mouse to capture the click sounds. 22 mouse clicks were carried out to move the target away from the upright position and trigger the bell sound. The mobile recorder captured the click sounds, while the WASAPI recorder captured the triggered bell sounds.

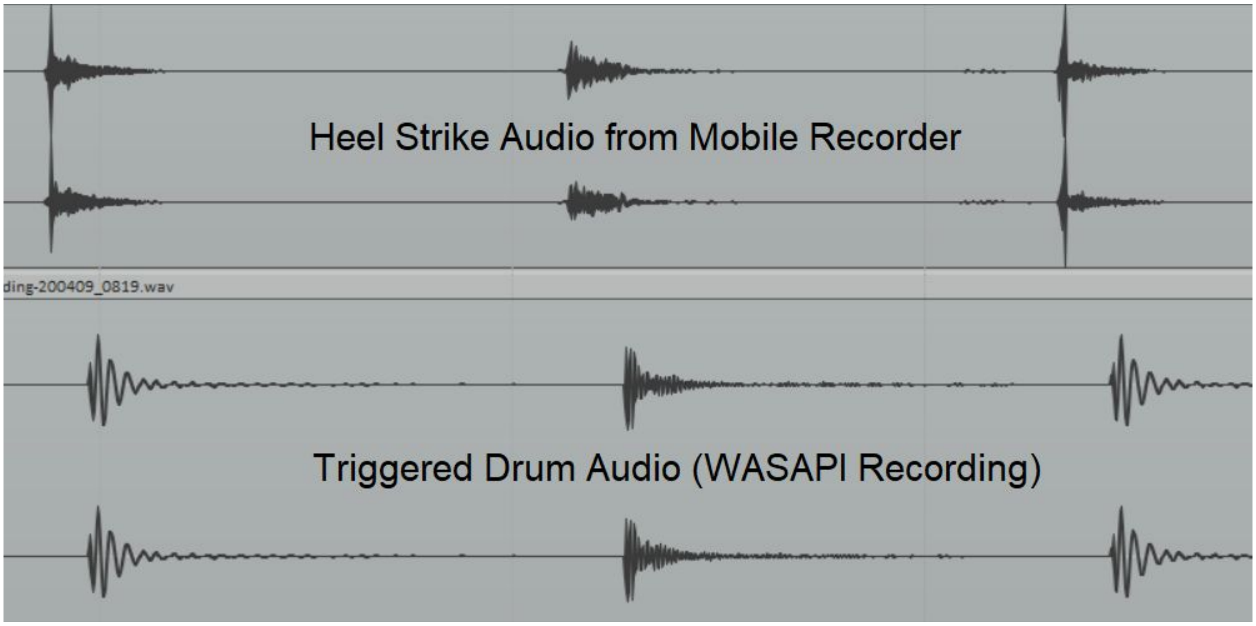


*Data Analysis*

In both cases, the WASAPI-recorded and mobile-recorded audio tracks were synchronized in a REAPER project by aligning the physical onsets of the leading sine bursts in each using

REAPER's *tab to transient* functionality, which detects physical onsets with high temporal accuracy. This functionality was then used to manually detect event timestamps of both the physical actions (clicks/steps) and its corresponding triggered feedback (bell/drums). Corresponding timestamps were compared and averaged to yield mean overall loop delay.

*Results*

Foot Strike: 93 +/- 48 ms
Trunk Angle: 90 +/- 5 ms

*Discussion*

In both cases, the loop delay measurements are relatively consistent and well below the documented human auditory reaction time, which is the requirement for concurrent biofeedback. The foot strike measurements show greater variability, possibly due to differences in step patterns and resulting accelerometer signals, which may have led to the events being detected slightly earlier or later with respect to the foot-strike audio transients. A limitation of this approach is that it does not give a finer picture of the stage-wise accumulation of delay. Also, the use of the mobile recorder does not account for sound propagation delays (although distances are short and these delays do not exceed 1-2 ms in any case) or transducer phase delay. A limitation of the mouse-click approach is that it does not account for delays incurred in the orientation computation process, as the sensor orientation is kept constant throughout the test. However, the sensor-fusion algorithm used does not perform any filtering (except a single sample averaging of gyroscope values), and the IMU smoothing filters do not incur a significant phase delay in the movement frequency range, so these delays are probably negligible.
