# Supplementary material for: A Technical Framework for Musical Biofeedback in Stroke Rehabilitation
Source: arXiv:2012.00323 source file (2020-12-01)
Supplement: Supplementary file 3 [file Supplementary_Material_3_-_Expert_Interview_Structure.pdf]

Thank you for agreeing to participate in the evaluation of the technology developed for my MSc thesis. The technology is a hardware and software prototype that is meant to provide user-customizable musical biofeedback to stroke patients during balance and gait rehabilitation.

<u>It does the following:</u>
A) measures different movement parameters while training with a **light wireless motion sensor**.
B) generates user-tailored computer music.
C) provides movement feedback through various changes in the music.

There are a number of *movement-music interaction possibilities* which are designed for the following types of training:

1) Static Upright Balance *(Posture Feedback)*
2) Trunk Control *(Trunk Position Feedback)*
3) Sit-to-Stand *(Jerkiness Feedback)*
4) Sit-to-Stand *(Trunk Angle-based Cue for Sitting and Standing)*
5) Gait *(Walking Rhythm Feedback)*

I now need your help to evaluate the above five movement-music interactions from the perspective of a clinician and a patient.

**<u>How will the interview be conducted?</u>**
The interactions will be demonstrated through the following videos (one for each). Each video is *<u>3-4 minutes</u>* in length. If you are curious, you are welcome to look at them, *but it is **not** necessary beforehand - time has been allocated for watching them during the interview*.

**https://youtu.be/PieRE05-3r8**
**https://youtu.be/q9uCmaBOzwU**
**https://youtu.be/fbi6YX-fClY**
**https://youtu.be/lWleA5t-yFg**
**https://youtu.be/ApNA6MsjlsM**

**The below questions will be asked for each interaction video.**
For all questions, constructive <u>critique</u> and <u>suggestions</u> for future improvement are greatly welcomed from your side.

*(Questions on next page)*

**Questions - Clinician Perspective**

Usefulness

Q1) Does the **sensing system** effectively capture the movement patterns relevant to this training activity?
Q2) Does the **music feedback** effectively convey patient movement information to the therapist during training?
Q3) Does the **music feedback** convey useful information about the patient that would not be available by conventional means (e.g. vision)?
Q4) To which specific impairment level of patients would this interaction be most relevant and useful?

Usability

Q1) Is this interaction suitable/adaptable to existing training protocols?
Q2) Please comment on the feasibility of this interaction from a real-life practical standpoint.
Q3) Are there other training situations where such an interaction could be used?

**Questions - Patient Perspective***

** Ideally would be asked to patients, but tests with them are impossible due to the current COVID19 situation. I request that you try to answer these on the behalf of the patient population, based on your experience.*

Usability

Q1) Does the feedback make sense in the context of the action that caused it? (intuitiveness, meaningfulness)
Q2) Would the feedback be easy for the typical patient to perceive?
Q3) Is the feedback given in a timely manner? (not too early/too late compared to the movement)
Q4) Would the patient's cognitive load be too high while doing the task?
Q5) Would the individual system adjustments help in covering the range of patient disabilities? What more can be adjusted to suit individuals?

AT END
Q1) Is the music enjoyable and motivating?
Q7) Would the hardware be comfortable to wear?
