# Supplementary material for: A Technical Framework for Musical Biofeedback in Stroke Rehabilitation
Source: arXiv:2012.00323 source file (2020-12-01)
Supplement: Supplementary file 4 [file Supplementary_Material_4_-_Expert_Interview_Results.pdf]

**Expert Interviews - Clinicians**

Due to the COVID-19 restrictions in Denmark during the planned final evaluation period with patients, these tests had to be cancelled. Instead, the interactions were evaluated through a series of expert interviews with music therapists and physiotherapists, all conducted remotely. The goal of these interviews was to obtain an expert assessment of the final set of developed sonic interactions, tackling the majority of the aspects that constitute the final problem formulation.

**Participants**

A total of seven experienced clinicians comprising five neurorehabilitation physiotherapists and two music therapists volunteered themselves for the interview. Of these, two of them had participated in previous iteration evaluations, and the remaining were approached for the first time, either independently or through AAU contacts. In terms of affiliations, one was attached to Neuroenhed Nord, Region Nordjylland, two to Hammel Neurocenter, Region Midtjylland, three to Kokilaben Dhirubai Ambani Hospital, Mumbai (India) and one to UCN.

**Setup**

All interviews were conducted over video-conferencing platforms such as Skype or Pexip Infinity Connect. Participants with a common affiliation were interviewed in groups, and all participants were hence covered over four sessions. The interactions were demonstrated through a series of videos shared with the participants as YouTube links (see 3.2.1 - 3.2.5 in https://docs.google.com/document/d/1GqhhQFhZWuepW9Ik-Qp4lHnRS0VcGtjc-p3nvbpeZvk/edit). The interviews were recorded with the permission of the participants using REAPER.

**Procedure**

All participants were provided with a brief information sheet beforehand, with details of the project and the interview questions (https://docs.google.com/document/d/1d6xWIIaIwsDIf-NhUBszqJzxnvC9M_ywlfrMFPY4m0/edit?usp=sharing). At the beginning of the interview, the structure was explained to the participants and they were requested to begin by watching the first sonic interaction video using a pair of headphones. When this was completed, they answered interaction-specific questions and this process was repeated for all five interaction videos in a fixed order. When the interviews were not one-on-one, the participants preferred to systematically divide the questions among themselves based on their individual areas of expertise.

**Data Analysis**

The interview recordings from REAPER were first transcribed (partially manually and with the help of DeIC Konch. The transcriptions were then coded by an inductive approach into a hierarchical coding scheme, illustrated in the figure. The three top level categories were *Clinician Usefulness, Clinician Usability and Patient Usability*. Within these, codes were assigned to sub-categories based on relevance. Themes were identified based on code incidence for each of the five sonic interaction videos, and these are summarized in the next subsection.

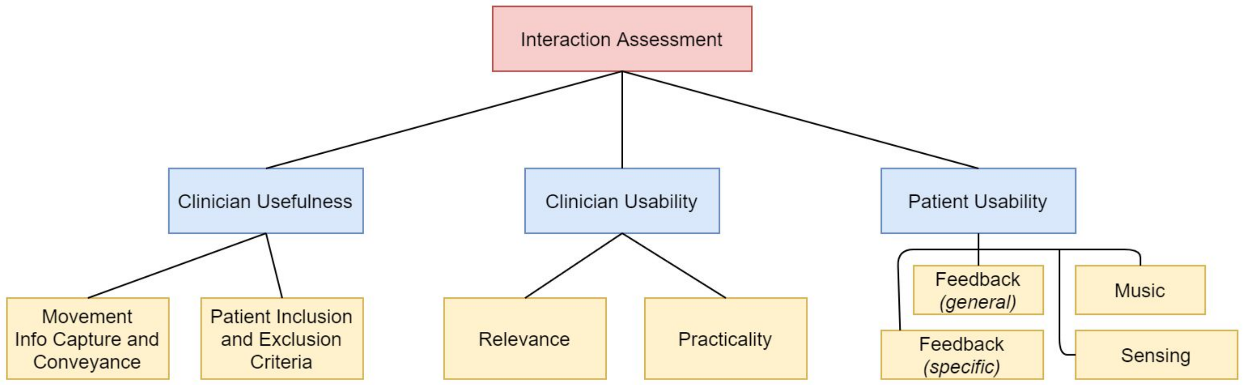


**Results**
The interview results are analyzed for each of the top-level categories of the coding hierarchy, specifically pertaining to each sonic interaction.

*(Abbreviations Used: SB = Static Upright Balance, DB = Dynamic Trunk Control, STS-Jerk = Sit-to-Stand (Movement Jerkiness), STS-Angle Cue = Sit-to-Stand (Movement Cues), Gait = Rhythmic Gait)*

**Clinician Usefulness**

Patient Inclusion and Exclusion Criteria

- Static Upright Balance (SB): The participants expressed that in general, patients with auditory perceptual difficulties and severe cognitive impairments would not be suitable for this form of biofeedback. One stated that candidates for musical biofeedback were those who are "unable to use tactile information from a therapist" to train balance, and those who are "motivated by music". Another mentioned that severely affected patients in particular could be easily confused by the feedback, which then "could be a minus", and that patients would "need some cognitive ability" to make use of it. Suggested target patient types were those with trunk stability problems, arm paralysis or neglect causing trunk tilt to the contralateral (paretic) side. Participants felt that this could potentially be used across physical impairment levels, ranging from acute/severe to moderate, although it would be less relevant as the patient's condition improves (e.g. if he/she begins walking).
- Dynamic Trunk Control (DB): Most participants felt that patients with trunk stability issues would be a suitable target group, but with better performance and flexibility than those that would be treated with the static balance interaction (SB), as dynamic balance exercises are typically more complex. One participant stated that sub-optimal spatial abilities would be a clear exclusion criterion. In terms of physical impairment groups, mild to moderate groups were stated to be more likely to benefit from this interaction as "acute patients with hardly any power would not be able to do the tasks" and as such, sub-acute or chronic patients could also be targeted.

- Sit-to-Stand - Movement Jerkiness (STS-Jerk): Participants generally felt that this would be most suited to "high-level" patients with the ability to independently sit and stand, as it would be difficult for moderately or severely impaired individuals to carry out the challenging STS weight transfer along with paying attention to the interaction. An example target group could be chronic stroke patients who have learnt the basic STS action "but would like to improve their movement quality".
- Sit-to-Stand - Movement Cues (STS-Angle Cue): Participants generally felt that patients needed to have good trunk stability in order to benefit from this interaction. One mentioned that "a patient progressing from acute to moderate, adequate trunk control, sitting control, little dynamic control is a perfect candidate – just above acute is a very good candidate". Another stated that it would be the same category as the STS-Jerk interaction with the ability to stand unsupported and fine motor control, although patients with memory problems would need to be excluded.
- Rhythmic Gait (Gait): Participants felt that inclusion criteria would depend not only on impairment severity but also on the location of the infarction/bleed. One provided a detailed explanation of how the typical effects of *cortical* strokes are stiffness and weakness, resulting in step time asymmetry and deviation from a straight line. The motor cortex plans movements and the basal ganglia coordinate their execution with the cerebellum. He continued that "RAS is commonly used in extrapyramidal conditions where power is normal but control is lacking. In cortical strokes, control is not lacking and the movement pattern is because of weakness and spasticity. The walking pattern can usually not be changed much with RAS like in Parkinson's Disease. Subcortical strokes with bleeding or infarcts of basal ganglia mimic Parkinson's Disease. Those patients are relevant to some extent but RAS will not work the same way for stroke patients as it does for Parkinson's Disease, broadly per se." Another participant concurred, mentioning that patients suffering from cerebellar or lower-brainstem bleeds, and thus having more cognitive ability but challenges with coordination, would be suitable candidates. Two participants expressed the concern that patients lacking rhythm-finding abilities would not be able to benefit from this interaction. In terms of physical impairment level, one participant stated that this would be "very attractive" to use with mild-moderately impaired patients who were at the stage of trying to stabilize gait aspects, a "useful and critical period where gait becomes more autonomous".

Movement Info Capture and Conveyance

- SB: The participants generally felt that the sensing system was able to capture relevant movement patterns away from the upright position both in the 3D space and the MLat and APos planes. They also felt that the biofeedback was effective at conveying this information to a therapist, but did not generally feel they received any new information about patient performance that vision would not provide. However, one participant mentioned that the information was more "exact" due to the fine nature of the measurements.
- DB: Here too, participants felt that the system effectively captured and conveyed the pertinent movement patterns owing to "the flexibility of the system and the feedback". While one participant did not feel that a therapist would receive additional information

from the auditory feedback, another mentioned that they "did get a movement sense from the feedback, which would be useful to know if the patient is about to reach the target position or has overshot it", while stressing that it was more important for the patient to receive this information than the therapist.

- STS-Jerk: Responses were more varied for this interaction. One participant felt that jerky movements were reliably sensed, but that the system seemed not to distinguish these from movements that were merely "fast or rapid". Multiple participants felt that the auditory feedback provided extra information that was not available visually, noting that the music captured subtleties of jerkiness better than the eye did, and that this information could be clinically useful in determining the stage of the movement at which patients tended to exhibit jerkiness. They felt that this could be added to the clinical information already available about the patient, and that the objective measurement of jerkiness could be useful in monitoring patient progress. However, one participant noted that this interaction did not capture trunk bend, a crucial STS variable. Others felt that although the knowledge of jerk was no doubt useful to obtain, they were unsure of whether the best course of action would be to directly provide feedback on it, or who might benefit from something of this kind. One participant explained that due to weakness, it is common for patients to use "trick" or "compensatory" movements in order to stand, and therapists are often required to use "momentum" to help patients stand, which can result in unavoidably jerky STS transitions. Negative feedback here would be confusing or discouraging to these patients.
- STS-Angle Cue: Participants generally felt that the sensing system was able to effectively capture the forward trunk bending motion. One highlighted that this could be very useful due to the importance of trunk bend to the STS transition and the usual inability of patients to gauge the optimal bend angle for standing and sitting, leading to them either falling backward when sitting or crashing back down when trying to stand. This participant stated that lower limb strength, trunk strength, patient balance, patient height and surface height were the main factors determining optimal trunk bend angles. Another mentioned that a therapeutic consideration is the strategy used by the patient in standing (hip or trunk), both of which are accounted for by the sensor. As far as conveying information to the therapist is concerned, one participant mentioned that the biofeedback did this effectively, although it was more important for the patient to receive this information.
- Gait: Participants felt that the system was effectively able to capture cadence and step patterns even in patients not having proper heelstrikes, although one pointed out that gait is indeed multidimensional. Another expressed that the emphasis of the interaction on heelstrikes would be good in focusing the attention of patients who tended to land on the forefoot or side of the foot. Two felt that this information was effectively conveyed to the therapist through the biofeedback, which provided extra information ("hearing the relation between the steps") whose acquisition would otherwise entail the recording and analysis of video footage.

**Clinician Usability**

Relevance to Existing Therapy Protocols

- SB: Participants generally felt that the interaction would fit well and could easily be integrated into both existing occupational therapy and physiotherapy protocols, with one also pointing out that the geometric system (circular/elliptical zones) corresponded well with what was used in regular training. A recurring theme in participant responses was an inclination towards using this interaction to provide continuous feedback while doing other tasks such as standing, sitting upright in one's room watching TV, reading the newspaper or bedside sitting during meals. Another possibility is in goal-oriented tasks with the purpose of monitoring trunk orientation while the patient does something with their legs or holds a training ball. It could also be used in occupational therapy tasks such as peeling apples or wiping a table. A participant also stated that this could be adopted in gait training by physiotherapists using the "Bobath" approach. Autonomy was stated by participants as an advantage in that it allows the patient to take charge in training their own static balance autonomously of the therapist, either alone or in groups. One participant compared this to existing dynamic posturography technology that uses visual feedback (e.g. Balance Master) and highlighted that this would be advantageous in terms of cost and portability while providing similar benefits.
- DB: There was good agreement that the interaction would fit well with existing protocols, given the abundance of goal-oriented reaching-related exercises in conventional therapy. One participant stated that its applicability could be widened by attaching the sensor to the upper limb or neck regions. Several felt that the concept could be adapted to create "fun training" scenarios, for example if the therapist too wears a sensor and conducts a "follow-me" exercise where the patient must mimic the movements of the therapist or if a visual component were to be added. One participant also stated that this too could aid patient autonomy in training by allowing the exercises to be done in groups with greater independence from the therapist.
- STS-Jerk: Participants similarly felt that this interaction would fit well with existing STS protocols and could easily be integrated. The participating therapist who had accompanied previous testing expressed that smoothness is important in all movements and indicates coordination; therapists want "timely and smooth setting in of muscles", relevant for STS. She also mentioned that this could be another "fun training" scenario, recalling the amusement of patients from Iteration 2 testing. Two participants mentioned that this interaction principle could also be used in a different task - providing feedback on hand or finger jerkiness while writing or drawing, as writing tremors are common among stroke patients.
- STS-Angle Cue: There was general agreement that this interaction would fit STS protocols, is relevant from an everyday therapeutic standpoint and could certainly be implemented in practice. One participant explained that a common practice is to have patients sit with one side against a wall having a vertical stripe that serves as a trunk bend STS cue, and that it would be interesting to see how this form of biofeedback would work instead of that. Another mentioned the possibility of greater patient autonomy as this would allow the patient to train STS anywhere independently, such as a chair in their own room. Adaptations of the interaction for other therapeutic purposes were also suggested, such as visual neglect, where a similar cueing sound could be

provided when a particular visual angle is scanned. It could similarly provide arm or shoulder angle biofeedback when training the upper limb (e.g. reaching exercises).

- Gait: Participants felt that this interaction would be useful to existing protocols (depending on whether the physiotherapist follows Bobath or evidence-based approaches). One stated that patients at all stages needed to train gait rhythm, and that body weight-supported systems could make such training possible even from very early stages of gait rehabilitation. Another (a music therapist) expressed the possibility of using the drum trigger interaction to provide PSE (patterned sensory enhancement) even in pre-gait training when the patient sits still and tries to raise his/her feet.

Practicality

- SB: A participant mentioned that a therapist would have to be mindful of and account for a short set-up time where individual-specific biofeedback parameters would have to be adjusted. Another asked whether it would be possible for the entire interface to be made available on a mobile device for easier and more portable use, and whether biofeedback settings for a patient could be saved for future recall.
- DB: One participant stated safety as a key concern here; the simultaneous need for a therapist to operate an interface while ensuring that the patient does not fall could lead to a usability issue, as therapists generally prefer to have their hands free. Solutions such as a body-mounted remote control or sensor (follow-me training) could address this issue. Participants agreed that in most cases, patient supervision would be necessary to prevent injury. Concerning the interaction, one participant mentioned that diagonal movements (MLat + APos) are an important focus of training, while the available controls only allow target zone manipulation in one plane at a time. A topic of disagreement was whether the interaction can be used without showing patients a visual interface of the target zone. Some felt it was necessary, while others felt that the combined sensory information may cognitively overwhelm the patient.
- STS-Jerk: Safety concerns and the need for supervision were similarly mentioned by one participant for this interaction, as the possibility of patients falling back down on the seat could be dangerous. Another mentioned that the jerk interaction might not be feasible in cases where the therapist uses "momentum" to help the patient stand, which would result in avoidable rapid and jerky movements and trigger negative feedback in an unfair manner.
- STS-Angle Cue: There were no further comments on practicality regarding this interaction.
- Gait: One participant stressed patient safety as an important concern, saying that this type of gait training is tough as patients must attend to the music rhythm and can get carried away in trying to follow the music even though they lack the balance to safely do so - it is thus safer to use body weight-supported systems. Another participant discussed practical problems with treadmill training due to the complexity of having to set a treadmill speed appropriate for the cadence and step length of the patient. A third mentioned the possibilities of using different musical meters to train distinct gait patterns, be they purely bipedal or with a cane/walker.

**Patient Usability**

- SB: Pertaining to the music feedback in general, participants agreed that it was clearly perceptible, provided in a timely manner and that the individual zone size adjustments would account for the inherent variability in patient impairments. One participant elaborated that "most stroke patients eligible for balance training will have enough auditory comprehension, except those with global aphasia who won't be taken for training – so patients who are amenable will be able to perceive the feedback". There was also agreement that the feedback made sense in terms of the action that caused it and would be intuitive for the patient as long as the therapist explicitly mentioned the goal of the interaction. Cognitive load, on the other hand, would depend on several factors, explained by one participant in terms of age, fatigue and cognitive ability. He stated that for example, a 60 year old stroke patient without dementia would be able to manage the interaction but a more elderly patient with dementia might not. Another mentioned that it would be up to the therapist to choose patients for whom this interaction would be most appropriate. The individual suitability of feedback strategies was also generally agreed upon. Several stated that they felt the ambulance strategy was "good" in that it managed to be clearly perceptible without being overly annoying, and that the directional feedback was helpful. One participant mentioned that while the melody distortion strategy was clear, it was very annoying and likely to put the patient off but testing would be necessary to gauge this. On the other hand, the cartoon effect was less annoying but more perceptually "blurred". Another mentioned that the feedback needed to be "somewhat annoying but not *so* annoying" as they were. A third expressed not liking the use of the word "punishment" as he felt the notion of punishing a stroke patient in any way was unethical.
- DB: In this case, participants agreed that the optimal music feedback strategy would vary among individuals depending on their perceptual ability, making it important for therapists to be able to choose between strategies. For example, two participants felt that the *Instrumentation* strategy was harder to perceive than the other clearer ones, meaning it would be more suited to "the higher end of patients". In general, they agreed that the feedback was provided in a timely manner, but differed on their preferred feedback strategy. One participant favored the *Music Stop* strategy, saying that the *Melody Detune - Frequency Distortion* was too annoying. Another favored the latter, as the former "did not reflect mild perturbations". Participants also agreed that the feedback was sensible and that the possibility to adjust the target zone size was very good. One participant mentioned that while this could be a "nice refreshing auditory exercise" for some patients, the cognitive load would depend on individual spatial abilities as some can find it difficult to orient themselves, but that it was otherwise generally "OK".
- STS-Jerk: Participants agreed that the auditory feedback is suitably adjustable, timely, sensible, and intuitive "smooth movement = smooth music - goes very well in the brain" as long as the therapist gives explicit instructions, although it would need to be tested. One appreciated the idea of providing positive reinforcement through pleasant sounding music, while another appreciated making this training more interactive as patients typically have to do hundreds of STS repetitions during their rehabilitation. While some felt the feedback was sufficiently clear, one felt that the feedback was "too fast" and that

the *Noise Disturbance (Scratch)* strategy was harder to perceive. Others favored the *Melody Tonic (Pitch)* strategy, saying that the *Noise Disturbance* was too annoying. In terms of patient cognitive load, one stated that it would depend on the awareness the patient has of their own jerky movements (falling down, for instance), saying the feedback would only be beneficial if patients lacked this awareness, otherwise it might create a "high" cognitive load.

- STS-Angle Cue: Participants agreed that while the feedback principle made sense, the choice of strategy would need to be individualized. Even in terms of their preferred strategy *Bell* v/s *Wah Wah*, participants disagreed considerably. Some favored the bell, citing reasons such as "it is an all-or-none movement so a single cue makes sense", "the bell provides a clear signal indicating the time to act", "the wah wah may not make sense to all" and "wah wah is annoying". Others favored the wah wah out of personal preference. Some participants did feel that the bell may be too soft for some patients to perceive along with the music, and asked whether it might be possible to control its volume level or simply amplify it. One participant felt that the cue "should be facilitating and not complex"; it would be most intuitive for the bell cue to be replaced by a human voice saying "Up" or "Down". Otherwise, participants agreed that the feedback was timely, the individual adjustments were sufficient and the cognitive load would be "OK" as long as the cues are perceptible.
- Gait: Between the two showcased interactions *Pitched Disturbance Punishment* and *Foot Drum Trigger*, participants generally favored the latter as "patients will always look for" positive reinforcement, which is "facilitating" and "supports motor learning", although it would need to be tested. Participants felt the feedback was clear, timely, suitably adjustable and intuitive, although some felt the *Pitched Disturbance Punishment* may be excessively annoying, especially if a patient must turn around in a small space or has rhythm-finding difficulties. Another felt that the difference between the left and right foot drum was not very large. While one felt the cognitive load would be manageable due to the intuitiveness of the feedback in general, another mentioned that some patients may lose track and need to be regularly reminded to pay attention to the feedback.

**Music**

Several participants highlighted the importance of subjectivity in terms of patient music preference and history of music consumption. One participant (a physiotherapist) felt it was enjoyable, but could not comment on its motivational value. Another (a music therapist) expressed that while the music was recognizable and engaging in that sense, it still sounded like computer music - some patients might not be bothered by alterations to their favorite music but for others, it is not that enjoyable. He speculated that this type of music would induce different affect and emotions than regular music while having a similar effect in terms of movement kinematics. While he appreciated the difficulty of the trade-off between control over music parameters and fidelity to the original, he concluded that it was simply "not the same". He also questioned the role of the music in, for instance, the STS Trunk Angle Cue interaction.

Another participant expressed that while music taste was highly subjective, music with a "low pulse" (slow tempo) might be more suitable to activities such as static balance or STS so as to prevent it from spontaneously inducing movement. Similarly, slow tempo music might also be suitable to gait rehabilitation where patients walk with a low cadence. Two participants who were familiar with previous iterations appreciated the variety added by introducing multiple music styles, saying it "was not as monotonous as last time", "it is important to have variety" and that it "absolutely does sound better than it did before".

**Wireless Sensor**

Participants agreed that it would be quite straightforward to strap on and that it would not add a significant practical overhead. One participant (accompanying physiotherapist from Iteration 2) expressed potential problems with using velcro as the strap material as it could potentially damage certain types of clothing materials (such as those used in sweaters) and suggested using elastic straps instead. She continued that hygiene could be a pertinent issue as well if the same sensors were to be used with multiple patients, and that they would have to be presented to the hygiene nurses for more details. Lastly, she asked whether the sensor could be "sewn into garments" or similar as we had experienced minor issues last time with foot sensors falling down mid-trial. Another participant mentioned that it was advantageous to be able to strap the sensor to the outside of clothing and not onto the skin directly, as some patients can find it "too close" or "annoying" when sensors are applied directly to the skin.
